# Supplementary material for: SWinGS: Sliding Windows for Dynamic 3D Gaussian Splatting
Source: arXiv:2312.13308 source file (2024-07-18)
Supplement: Supplementary file 1 [file X_supp.tex]

\section{Video Results}
We present video results of our proposed method compared to the following SoTA methods: K-Planes~\cite{fridovich2023}, HexPlane~\cite{cao2023}, MixVoxels~\cite{wang2023}, HyperReel~\cite{attal2023}, NeRFPlayer~\cite{song2023}, StreamRF~\cite{li2022b}, and Dynamic 3D Gaussians~\cite{luiten2024}, in a video entitled  \textcolor{blue}{07170-supp-video.mp4}, which is included in the zipped folder. We demonstrate noticeable improvements over the competing methods, with sharper and more detailed renderings and fewer temporal artifacts. We encourage viewing the video results to fully appreciate the quality improvements provided by our method. The video also shows examples of novel view synthesis, the effects of temporal consistency fine-tuning and regular vs dynamic MLPs, and an example of our interactive dynamic viewer.

\section{Implementation Details}
Here, we discuss additional implementation details that enable our method to produce high-quality renders of dynamic scenes from multi-view data.

\subsection{Tunable Dynamic MLP Implementation}
\label{sec:mlp_implementation}

As discussed in section~\textcolor{red}{3.5}, key to our approach are tunable dynamic MLPs~\cite{Maggioni2023TunableCW} with additional learnable blending parameters $\boldsymbol{\alpha}$. This formulation enables disentanglement of static and dynamic parts of the scene by focusing the MLP on the dynamic parts, while temporally-local canonical sets of Gaussians model the start parts (\ie two ``motion modes''). The learnable blending weight $\boldsymbol{\alpha}$ essentially weighs the MLP parameters for each input Gaussian $i$ and is optimized as an additional model parameter.

To execute the dynamic MLP in PyTorch, we re-implement the linear layers of a regular MLP as a dynamic MLP using PyTorch's batch matrix multiplication, thus enabling efficient forward pass computation. We implement a single layer of a dynamic MLP as follows. For a single tunable linear layer, we have a matrix of $M$ sets of MLP weights $W^{M \times f_{in} \times f_{out}}$ and biases $B^{M \times f_{out}}$, with $f_{in}$ and $f_{out}$ input and output features, respectively, for a set of blending parameters $\{\alpha^m_i\}^M_{m=1}$ governing $M$ modes of motion. The weights $W$ are initialized uniformly, and the biases $B$ are initialized to zeros. In our experiments, we learn two tuning parameters $\alpha_i$ ($M=2$) for each Gaussian $i \in N_g$ in the dynamic 3DGS model, therefore smoothly separating the scene into two modes: static and dynamic. During training, as the number of Gaussians densifies, we also similarly densify the $\boldsymbol{\alpha}$ parameters following the same densification procedure as 3DGS~\cite{kerbl2023}, \ie if a Gaussian is cloned or pruned, so is it's corresponding $\alpha$. The complete optimizable parameters $\theta$ of the dynamic MLP are thus:

\begin{align*}
    \theta = \{ W^{M \times f_{in} \times f_{out}}, B^{M \times f_{out}}, \boldsymbol{\alpha}^{N_g \times M} \}
\end{align*}

Reshaping and element-wise multiplying the blending parameters $\boldsymbol{\alpha}^{N_g \times M}$ with the MLP weights $W^{M \times f_{in} \times f_{out}}$ and biases $B^{M \times f_{out}}$, and summing over the $M$ dimension, essentially results in $N_g$ sets of dynamic weights $W_{\textrm{dyn}}$ and biases $B_{\textrm{dyn}}$, \ie a set of MLP parameters for each input Gaussian $i$, weighed by their corresponding blending parameters $\boldsymbol{\alpha}$:

\begin{align*}
    W_{\textrm{dyn}}^{N_g \times 1 \times f_{in} \times f_{out}} &= \sum_M \boldsymbol{\alpha}^{N_g \times M \times 1 \times 1} \cdot W^{1 \times M \times f_{in} \times f_{out}}\\
    B_{\textrm{dyn}}^{N_g \times 1 \times f_{out}} &= \sum_M \boldsymbol{\alpha}^{N_g \times M \times 1} \cdot B^{1 \times M \times f_{out}}
\end{align*}

To compute the outputs $\boldsymbol{y}$ of a single layer of the dynamic MLP with a single forward pass, the frequency-encoded inputs $\gamma(\boldsymbol{x})^{N_g \times f_{in}}$ are reshaped and batch multiplied with the set of dynamic weights $W_{\textrm{dyn}}$ before being summed with the dynamic biases $B_{\textrm{dyn}}$. The output is then passed through the activation function $\phi$:

\begin{equation}
    \boldsymbol{y}^{N_g \times 1 \times f_{out}} =\\
    \phi \left(
    \textrm{bmm} \left(
    \gamma(\boldsymbol{x})^{N_g \times 1 \times f_{in}}, W_{\textrm{dyn}}^{N \times f_{in} \times f_{out}} \right) + 
    B_{\textrm{dyn}}^{N_g \times 1 \times f_{out}}
    \right)
\end{equation}

\subsection{Hybrid Training Strategy}

Our method incorporates a two-stage hybrid training strategy to achieve high-quality rendering performance and temporally consistent novel views. Firstly, we independently train dynamic 3DGS models for each window in the sequence. This is done in parallel across 8 NVIDIA Tesla 32GB GPUs, allowing faster training. Secondly, we ensure temporal consistency by fine-tuning each model sequentially. In this stage, we use a single GPU, as the model of the previous window is required to fine-tune the current window. Therefore, this stage in our current implementation cannot be performed in parallel. However, this is an aspect we aim to improve in future work.

\section{Evaluation}

To the best of our knowledge, there are only a few publicly available multi-view datasets of general dynamic scenes. Many are human-centric rather than general scenes, which may be better served with template-based methods (\eg SMPL). Our model is specifically non-template-based to handle generic scenes. Furthermore, our method is designed for multi-view static camera setups (\eg LightStage) and thus, we do not consider monocular datasets, which is in essence a different problem~\cite{gao2022dynamic}. For these reasons, we focused on two main multi-view dynamic benchmarks for our evaluation: the Neural 3D Video dataset~\cite{li2022a} and Technicolor~\cite{Sabater2017} dataset. We considered the Immersive Light Field Video dataset~\cite{broxton2020immersive}; however, this dataset comprises heavily distorted fish-eye lenses and inconsistent imaging parameters across views. Inconsistent exposures/white-balance differences can be handled following recent works by learning per-image appearance embedding~\cite{martinbrualla2020nerfw}, but this is not the focus of our paper.

\subsection{Neural 3D Video Dataset}

The Neural 3D Video dataset~\cite{li2020} is captured with 21 cameras at 30fps at a resolution of $2704 \times 2028$. It mostly consists of indoor activities in various lighting conditions. Following previous works, we downsample images to half resolution of $1352 \times 1014$ in our experiments. We follow the training and validation camera split provided by~\cite{li2022a}, evaluating on the central camera over six different scenes. We provide additional qualitative results in Fig.~\ref{fig:n3d_results_supp} with close-up crops highlighting significant differences. Our method produces noticeably sharper renderings compared to the other methods with fewer artifacts. Please find our supplementary video for more results and sequence visualisations.

\subsection{Technicolor Dataset}

The Technicolor dataset~\cite{Sabater2017} is captured with 16 cameras in a $4 \times 4$ grid at 30fps at a resolution of $2048 \times 1088$. We follow the same evaluation procedure and training and test splits of HyperReel~\cite{attal2023}, evaluating on five scenes at full resolution, where the test camera is at the second row second column. We provide additional qualitative results in Fig.~\ref{fig:technicolor_results_supp} with close-up crops highlighting significant differences. Again, similar to our results on the Neural 3D Video dataset, our method produces generally sharper renderings compared to the other methods, with strong temporal consistency and fewer artifacts. Please find our supplementary video for more results and sequence visualisations.

\section{Limitations}

Although our method has demonstrated impressive results, we would like to highlight a few limitations.

Our current approach to adaptive window sampling involves dividing the sequence into sliding windows based on predetermined thresholds. Once the sum of the mean optical flow magnitude across all camera views hits this threshold, a new window is created. However, this threshold must be manually set for each sequence to ensure that motion is evenly distributed across models. At present, we determine the optimal threshold through experimentation. If the training performance (PSNR) is not satisfactory, smaller windows are needed to capture motion, and a lower threshold is required (leading to more frequent window sampling). Conversely, if training PSNR is high, fewer windows may suffice, and a higher threshold could be used, requiring fewer models to be trained and reducing training overhead by saving computational time and model storage. Going forward, we aim to eliminate this heuristic by learning the optimal threshold in a differentiable manner. This is an area we plan to address in future work.

The quality of the resulting renders for novel views is greatly influenced by the number of frames in the sampled windows, taking into account the amount and complexity of motion in the scene. This factor is also determined by the frame rate at which the sequence is originally captured. In other words, the greater the distance between moving objects in neighbouring frames, the more challenging it is for the MLP to learn the Gaussian displacements. To tackle this complex issue, a coarse-to-fine training strategy can be employed, starting at a lower resolution and gradually increasing the resolution during training. Alternatively, a voxel grid-based model may be used, coupled with a coarse-to-fine strategy.

\begin{figure}
\captionsetup[subfigure]{labelformat=empty}
\centering
\begin{tabularx}{0.9\linewidth}{
l @{\hspace{0.85\tabcolsep}} 
c @{\hspace{0.85\tabcolsep}}
c @{\hspace{0.85\tabcolsep}}
c @{\hspace{0.85\tabcolsep}}
r}
\subfloat[MixVoxels]{\includegraphics[width = 0.17\linewidth]{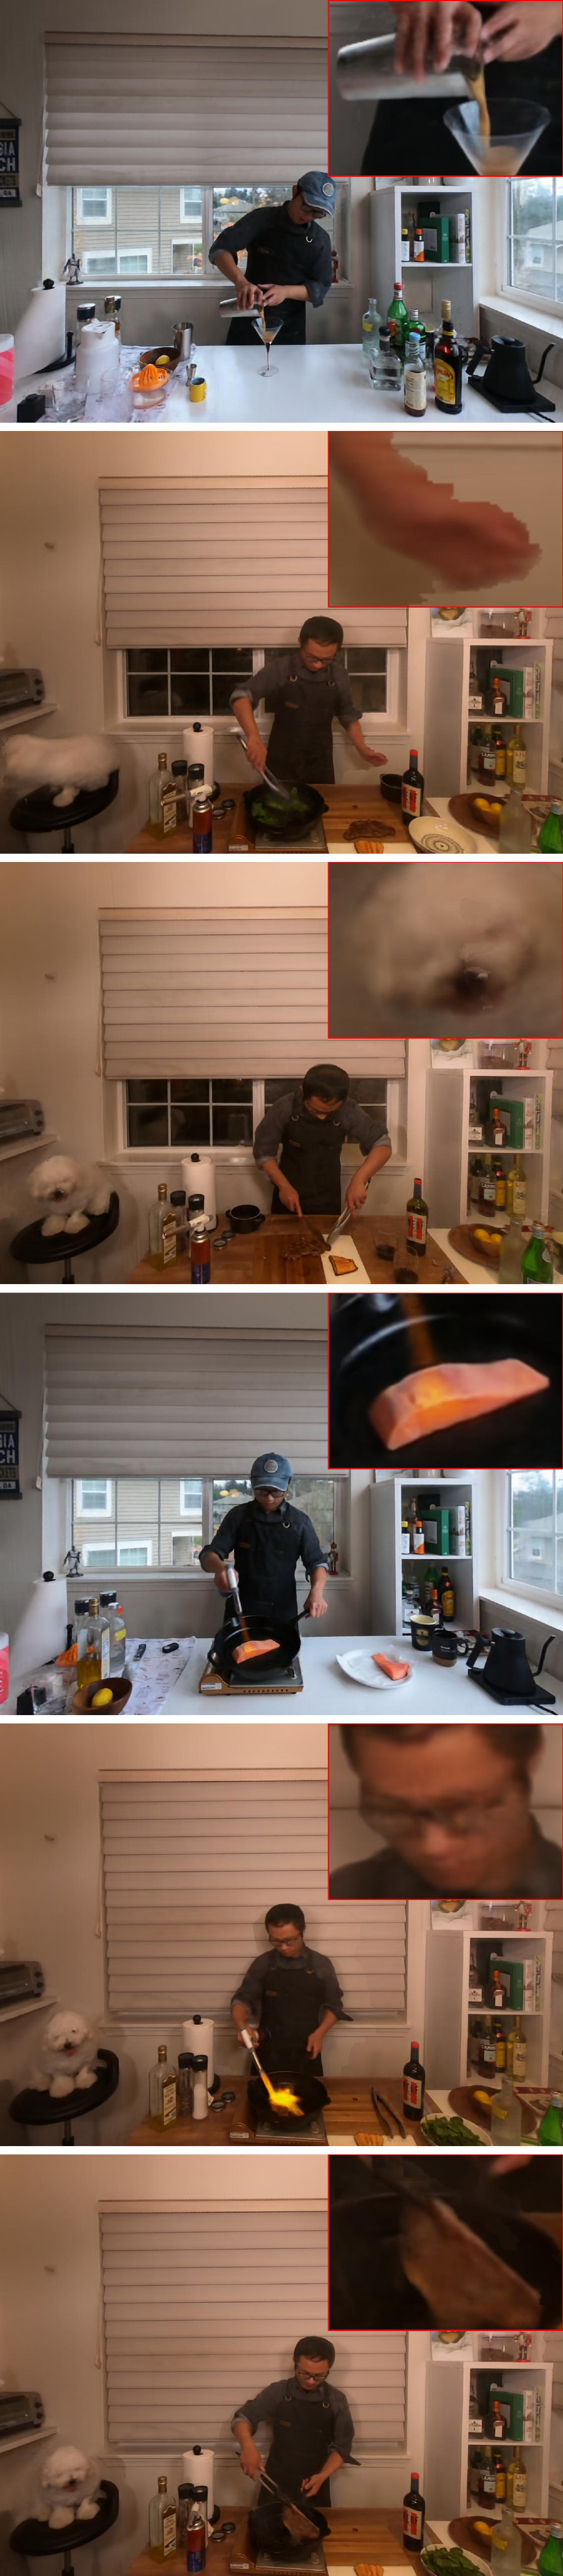}} &
\subfloat[K-Planes]{\includegraphics[width = 0.17\linewidth]{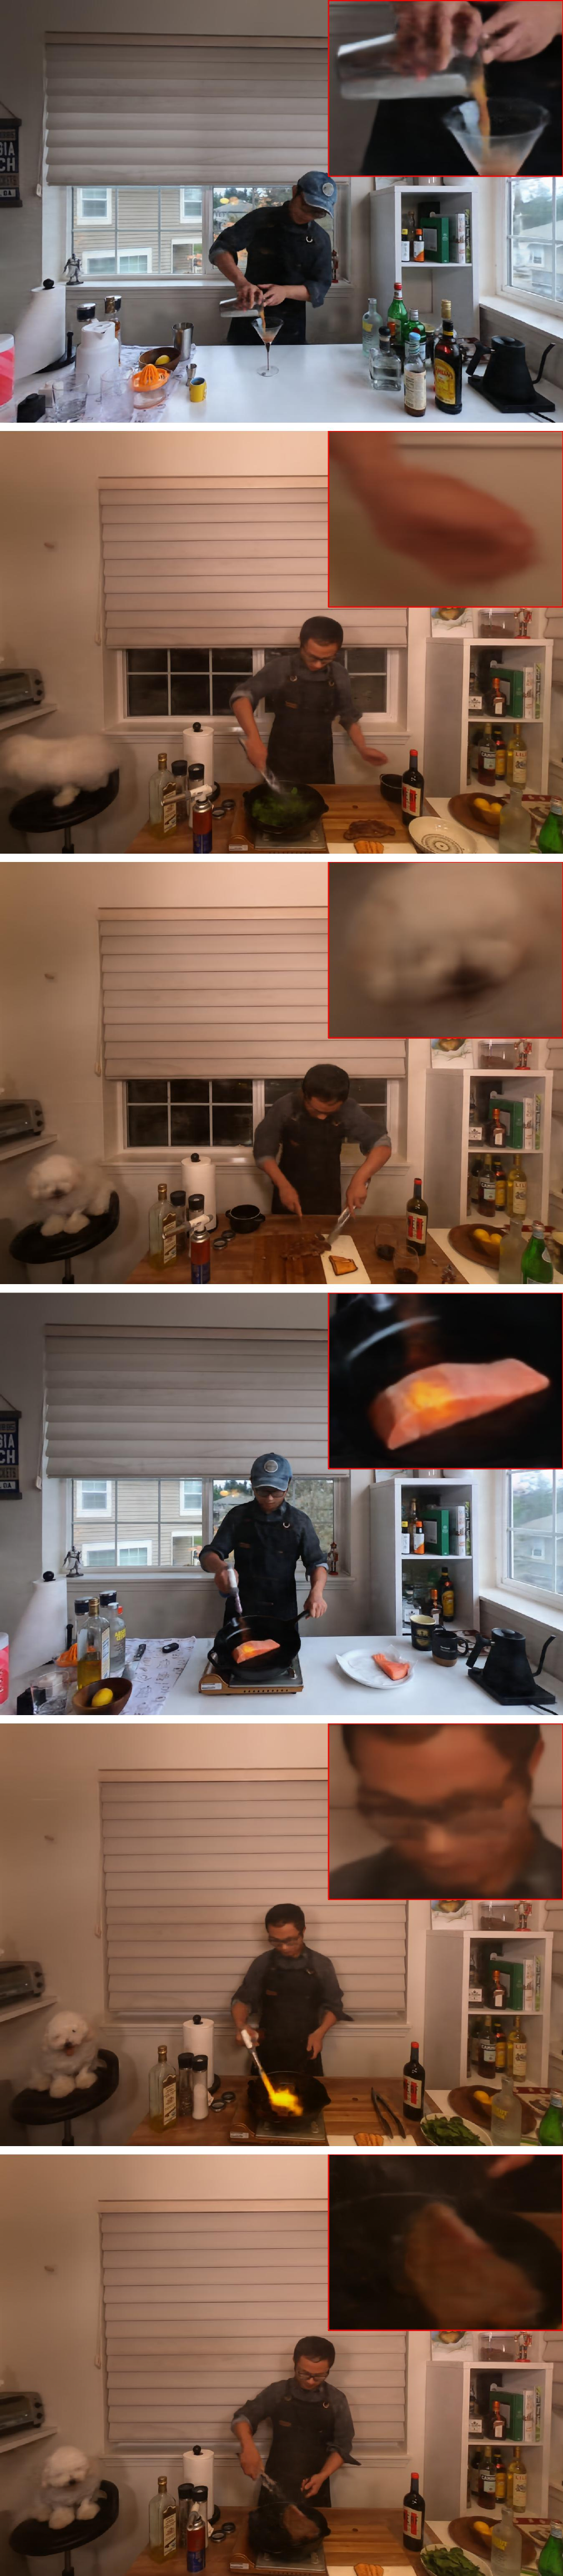}} &
\subfloat[HyperReel]{\includegraphics[width = 0.17\linewidth]{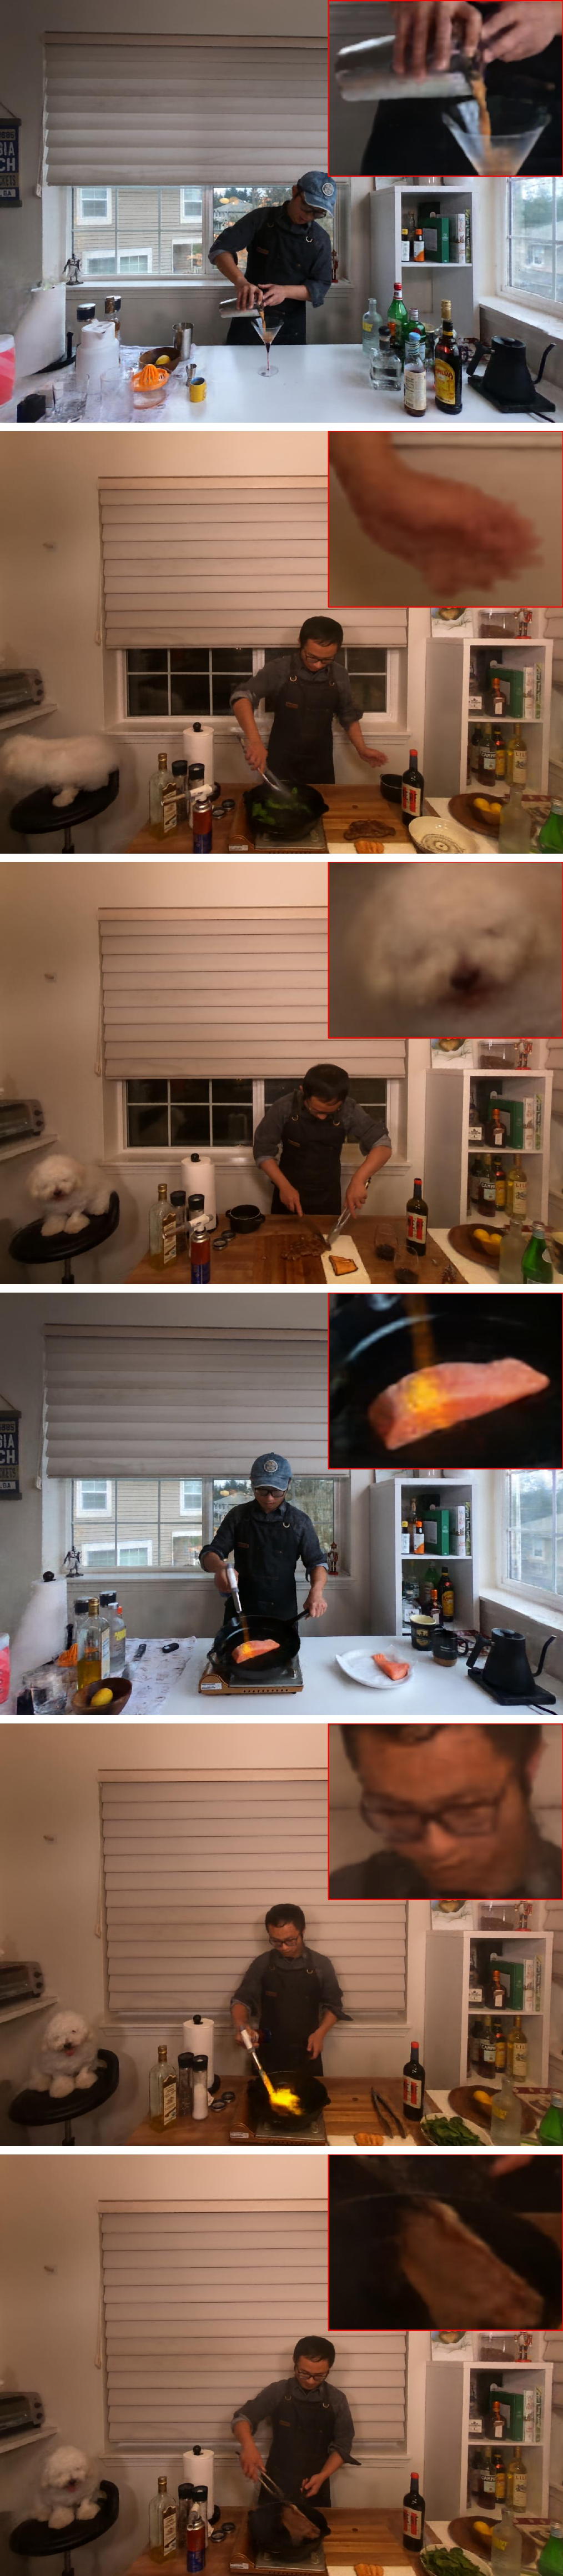}} &
\subfloat[\textbf{Ours}]{\includegraphics[width = 0.17\linewidth]{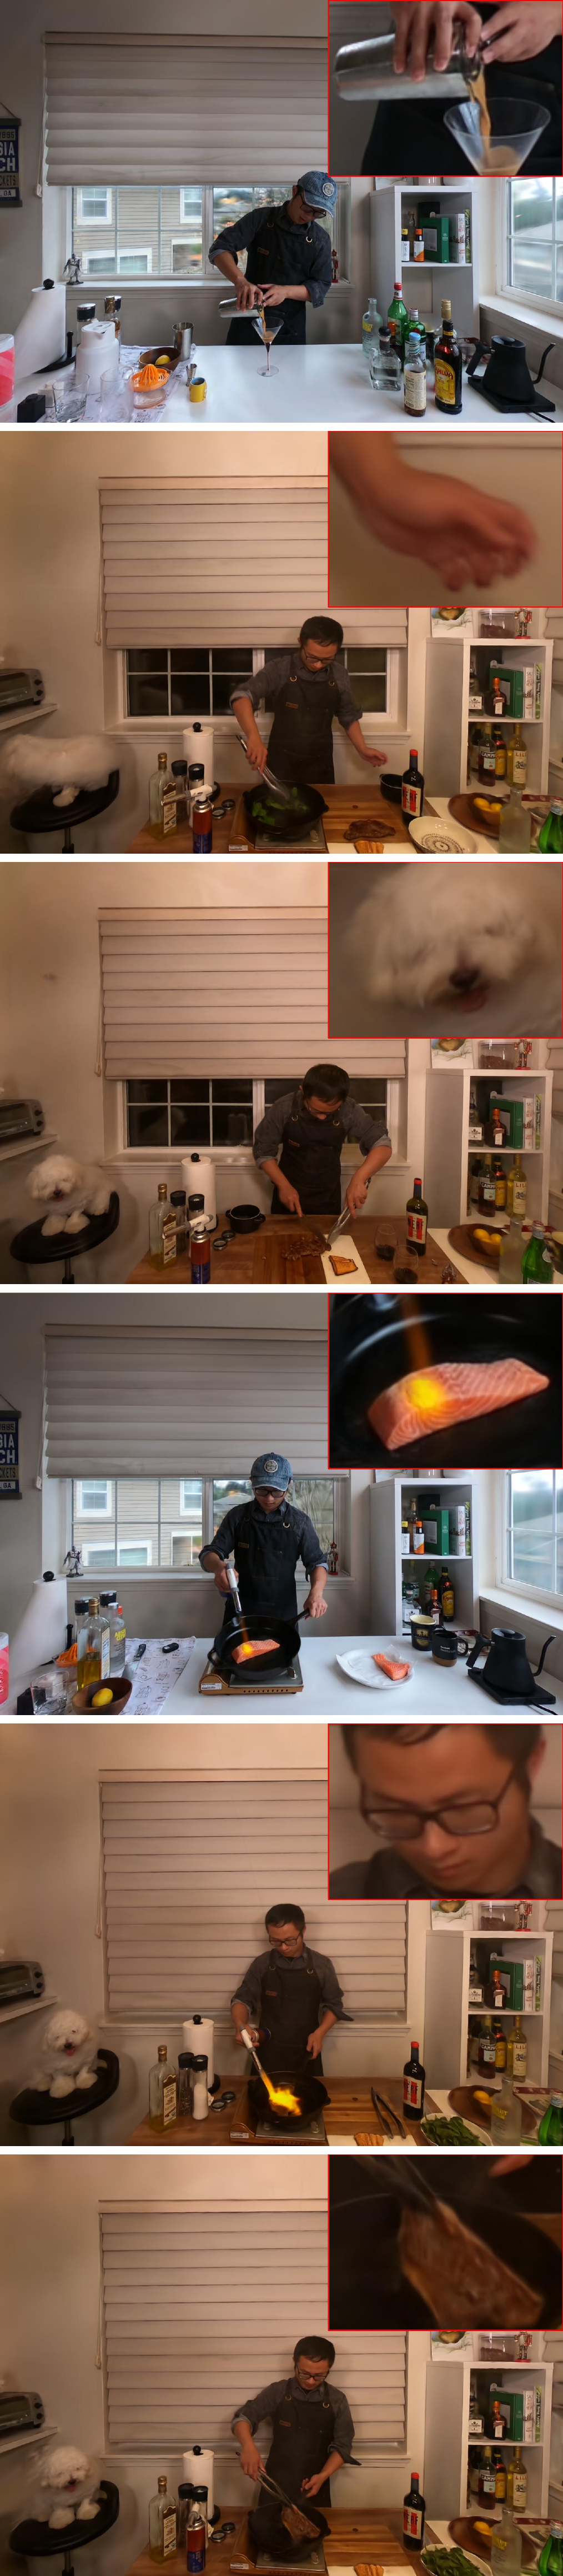}} &
\subfloat[Ground truth]{\includegraphics[width = 0.17\linewidth]{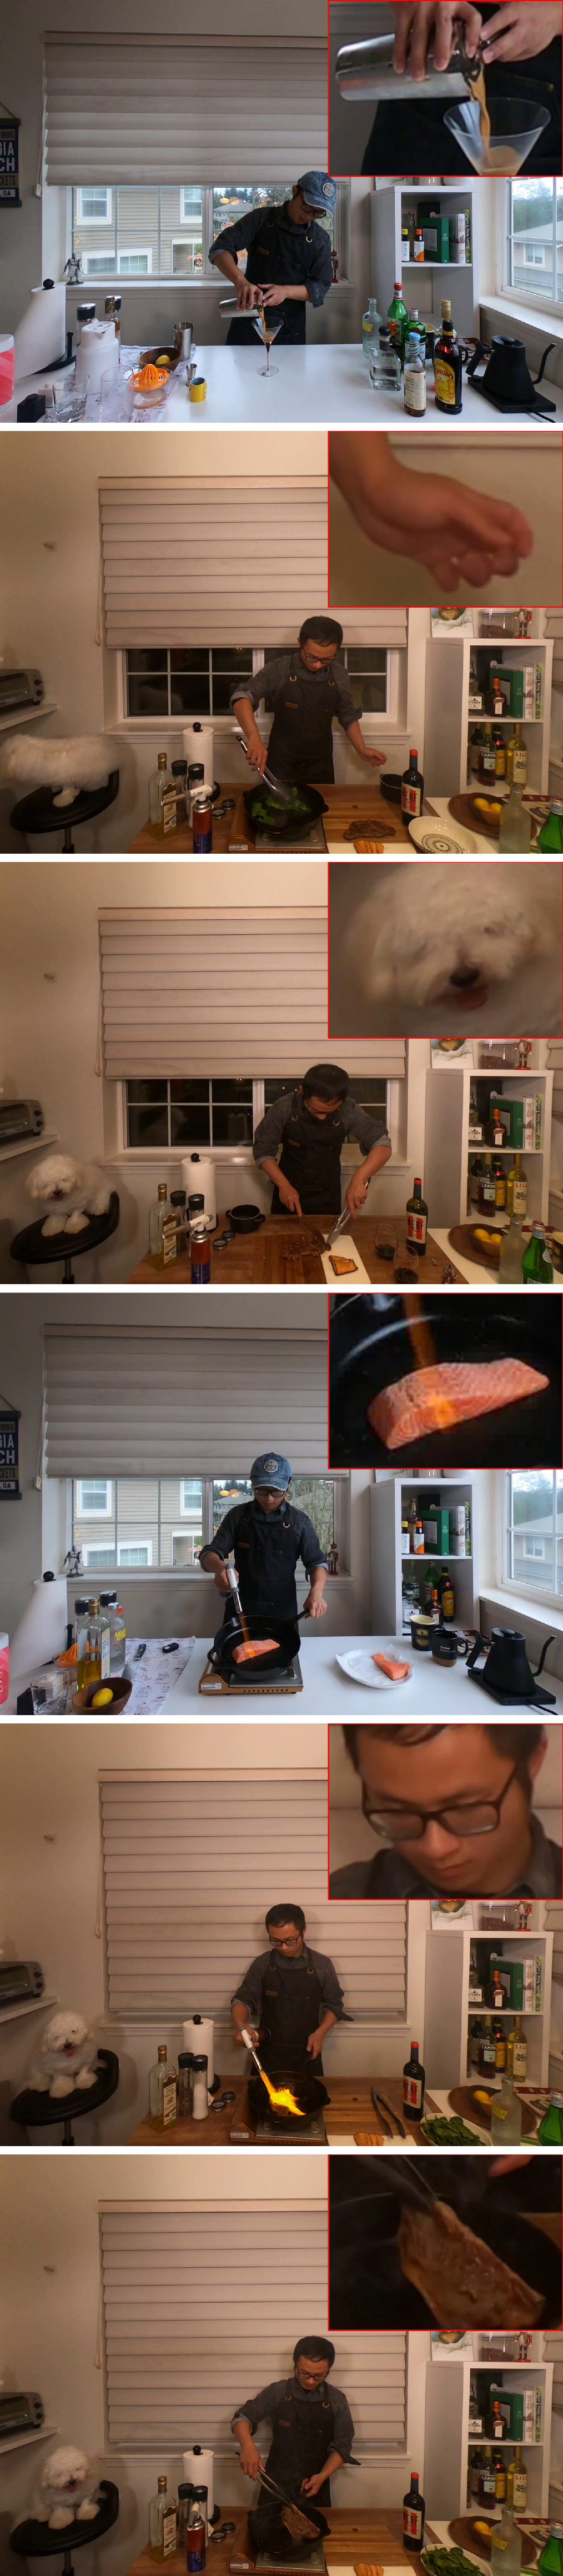}}
\end{tabularx}
\caption{Additional qualitative results on Neural 3D Video~\cite{li2022a}. Scenes top to bottom: i) \textit{coffee martini}, ii) \textit{cook spinach}, iii) \textit{cut roasted beef}, iv) \textit{flame salmon}, v) \textit{flame steak}, and vi) \textit{sear steak}.}
\label{fig:n3d_results_supp}
\end{figure}

\begin{figure}
\captionsetup[subfigure]{labelformat=empty}
\centering
\begin{tabularx}{0.88\linewidth}{
l @{\hspace{0.85\tabcolsep}} 
c @{\hspace{0.85\tabcolsep}}
c @{\hspace{0.85\tabcolsep}}
r}
\subfloat[HyperReel]{\includegraphics[width = 0.21\linewidth]{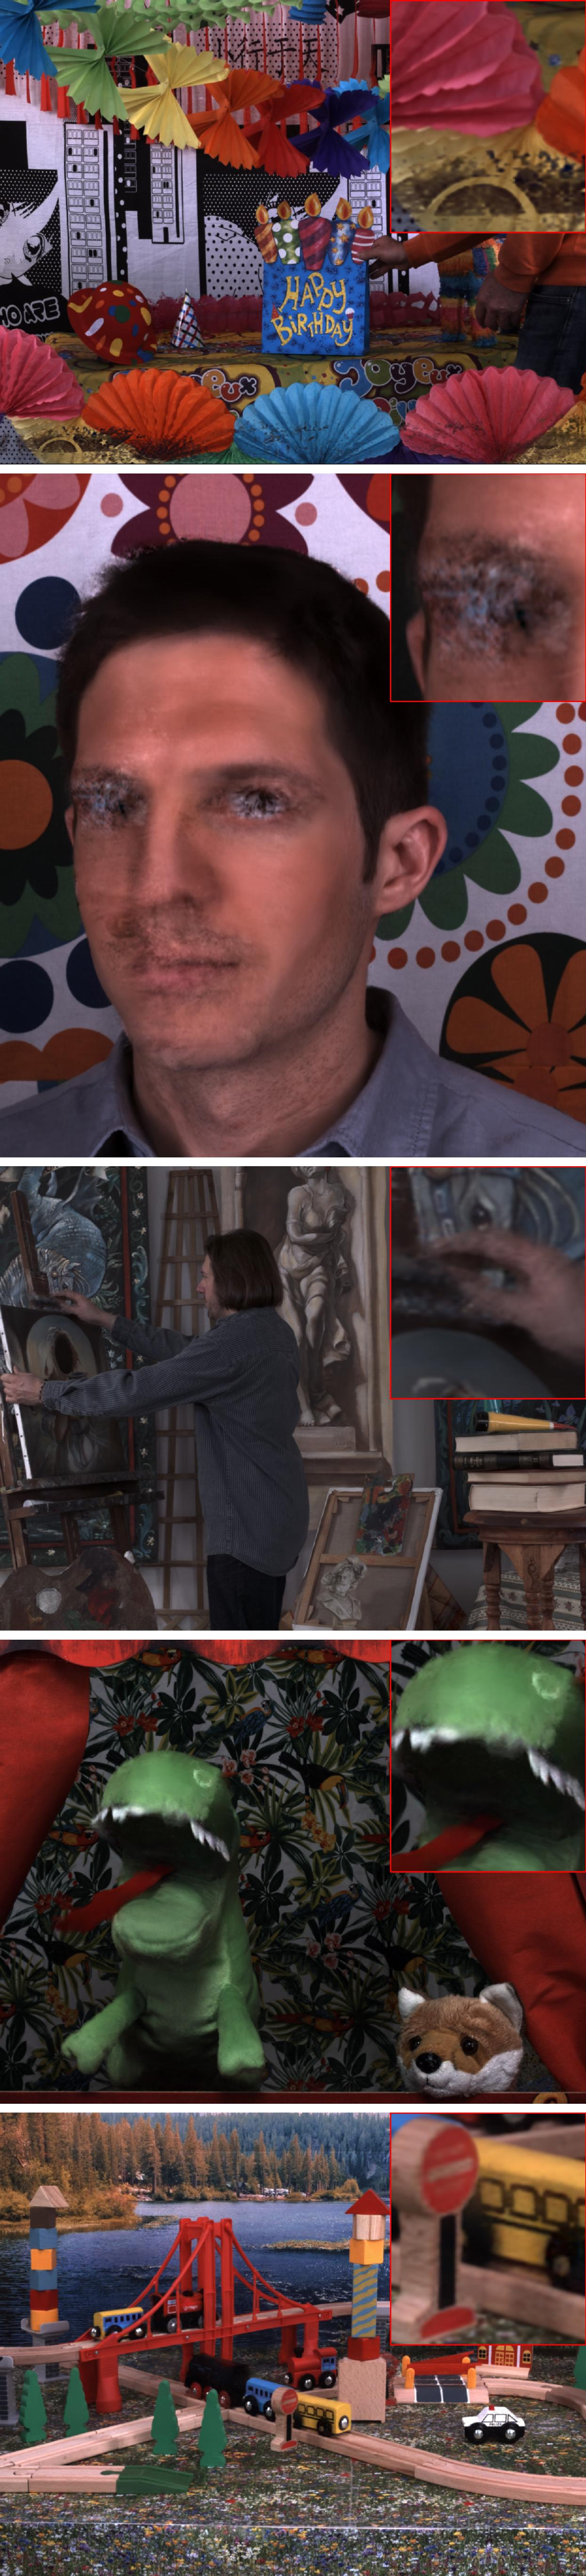}} &
\subfloat[Dynamic3DG]{\includegraphics[width = 0.21\linewidth]{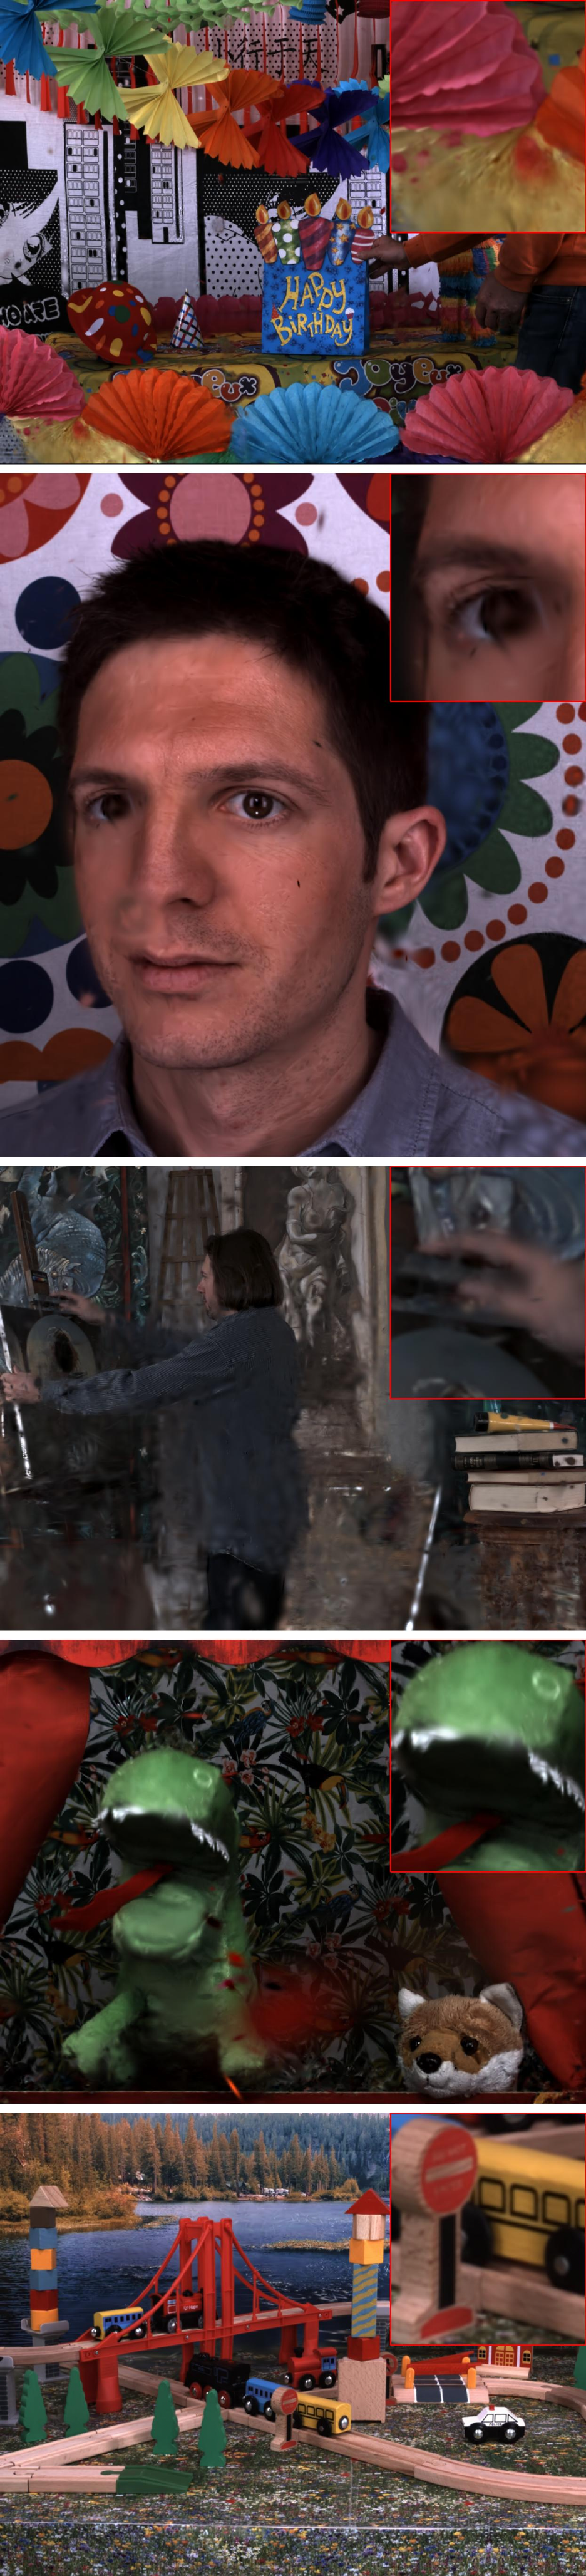}} &
\subfloat[\textbf{Ours}]{\includegraphics[width = 0.21\linewidth]{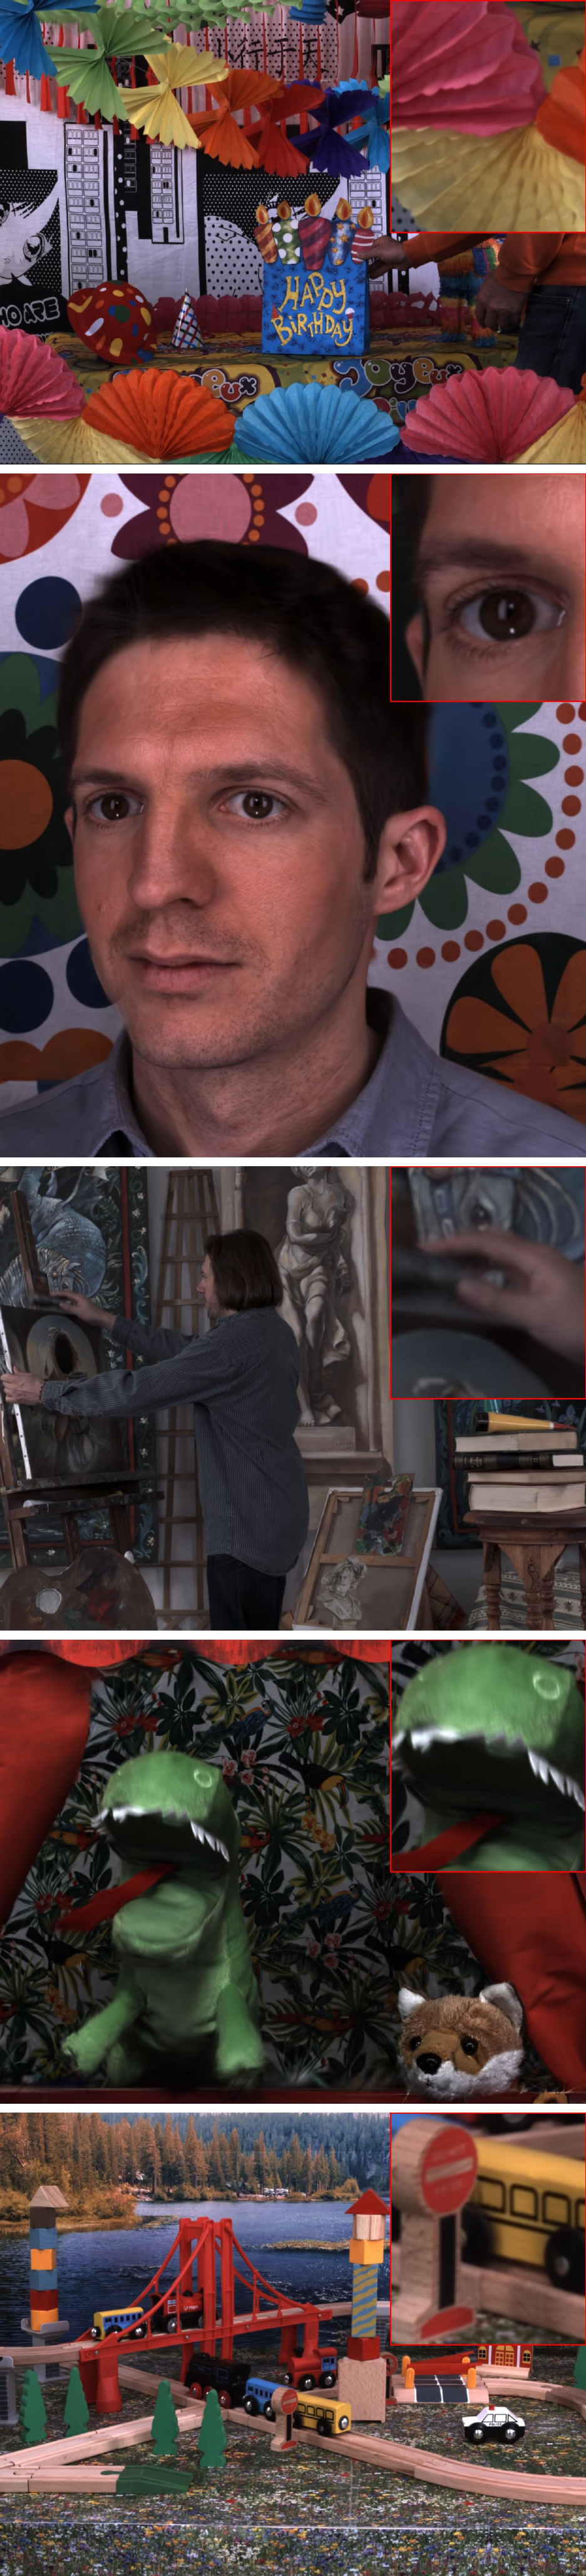}} &
\subfloat[Ground truth]{\includegraphics[width = 0.21\linewidth]{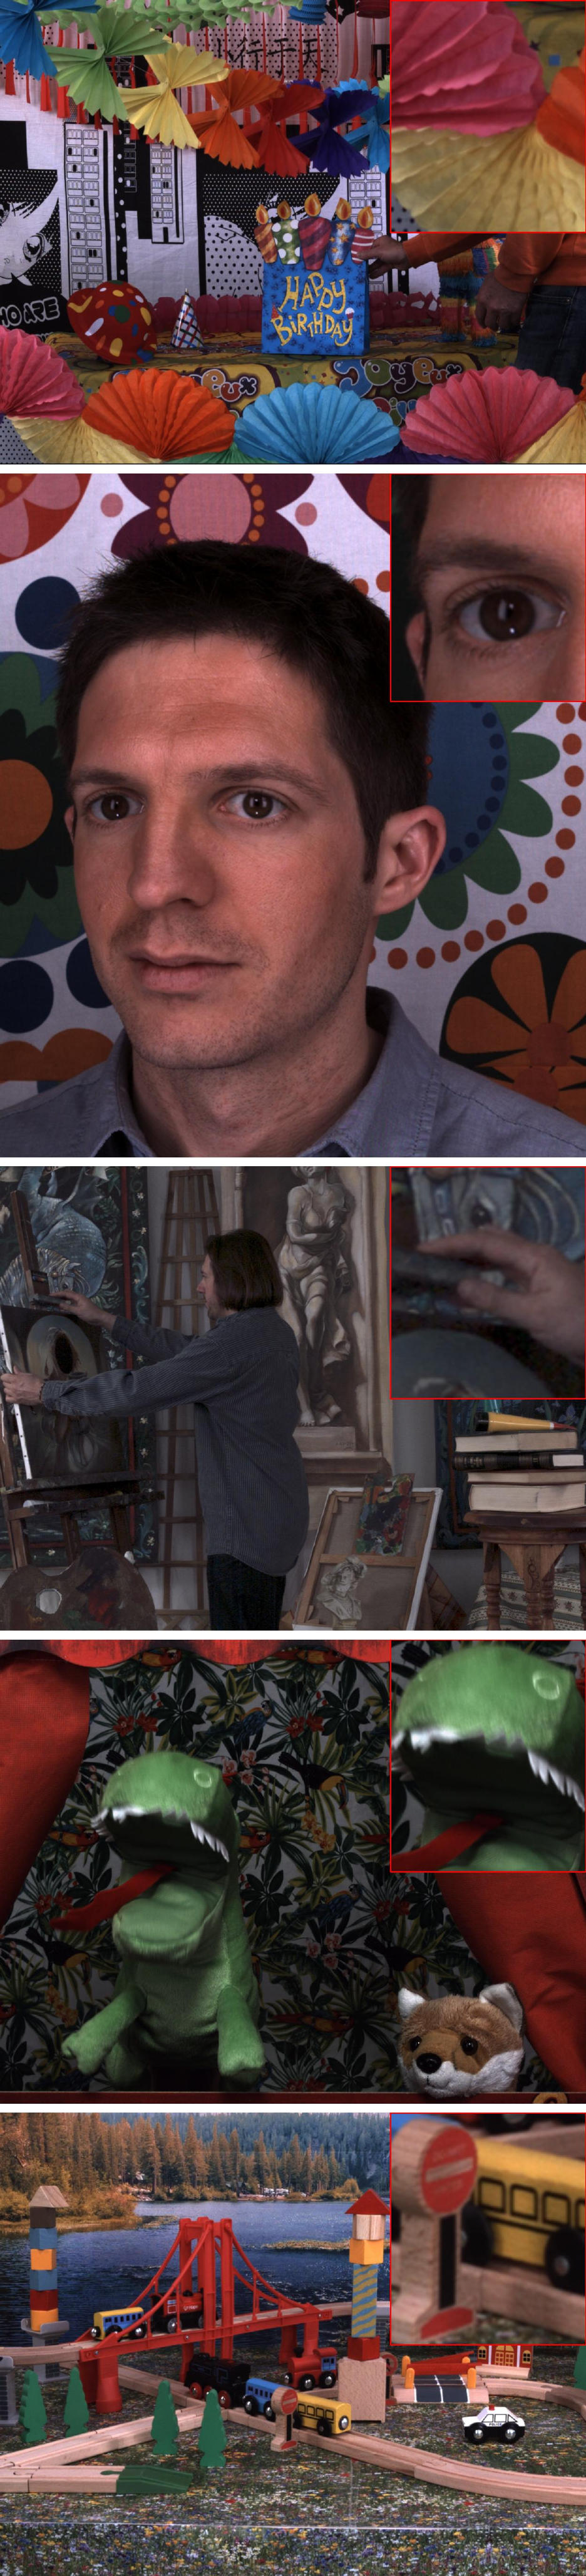}}
\end{tabularx}
\caption{Additional qualitative results on Technicolor~\cite{Sabater2017}. Scenes top to bottom: i) \textit{Birthday}, ii) \textit{Fabien}, iii) \textit{Painter}, iv) \textit{Theater}, and v) \textit{Train}.}
\label{fig:technicolor_results_supp}
\end{figure}
